# Supplementary material for: Learning from weakly dependent data under Dobrushin's condition
Source: arXiv:1906.09247 source file (2019-06-21)
Supplement: Supplementary file 1 [file uc-appendix.tex]

\section{Uniform convergence related stuff}

\section{Proving $\varepsilon$-representativeness.}
.\yuval{Move to the appendix / main body}

Given a training distribution $D^{(m)}$ over $(X\times Y)^m$, a test distribution $D$ over $X\times Y$ and a hypothesis class $H$, one is usually interested in finding
$0 < \varepsilon, \delta < 1$ such that $\rv{S} \sim D^{(m)}$ is $\varepsilon$-representative with probability $1- \delta$ with respect to the test distribution $D$.
In particular, we would like to show that
\[
\Pr_{\rv{S}\sim D^{(m)}} \left[ \sup_{h \in H} \left| L_D(h) - L_{\rv{S}}(h) \right| > \varepsilon \right] < \delta.
\]
It is usually easier to remove the absolute value, bounding both
\begin{equation}\label{eq:12}
\Pr_{\rv{S}\sim D^{(m)}} \left[ \sup_{h \in H}  \left(L_{\rv{S}}(h) - L_{D}(h)\right) > \varepsilon \right]
\end{equation}
and the second inequality using the same methods.
It takes two steps to bound Eq.~\ref{eq:12}:
first, the (usually) harder task is bounding the expectation
\begin{equation} \label{eq:bnd-exp}
\EE_{\rv{S} \sim D^{(m)}} \left[ \sup_{h \in H} \left( L_{\rv{S}}(h) - L_D(h) \right) \right].
\end{equation}
Then, bounding the deviation,
\begin{equation} \label{eq:16}
\Pr_{\rv{S} \sim D^{(m)}} \left[
\sup_{h \in H} \left( L_{\rv{S}}(h) - L_D(h) \right)
> \EE_{\rv{S}} \left[ \sup_{h \in H} \left(L_{\rv{S}}(h) - L_D(h) \right) \right] + t
\right],
\end{equation}
for all $t > 0$. The bound on the expectation is usually in terms of the Radamacher complexity, while the high probability bound is obtained using McDiarmid inequality.

Note that instead of considering a family $H$ of hypotheses, one can consider the family of loss functions $\cF = \{ \ell_h \colon h \in H\}$. The domain $X \times Y$ of the loss functions $\ell_h$ is replaced with a general $Z$. Then, \eqref{eq:bnd-exp} translates to
\begin{equation} \label{eq:17}
\EE_{\rv{S} \sim D^{(m)}} \left[ 
\sup_{f \in \cF} \left( 
\frac{1}{m} \sum_{i=1}^m f(\rv{s}_i) - 
\EE_{\rv{t} \sim D}\left[ f(\rv{t}) \right]
\right) 
\right]
= \frac{1}{m} \EE_{\rv{S} \sim D^{(m)}} \left[ 
\sup_{f \in \cF} \left( 
\sum_{i=1}^m f(\rv{s}_i) - 
\EE_{\rv{S}} \left[ \sum_{i=1}^m f(\rv{s}_i) \right] 
\right) 
\right],
\end{equation}
where the equality follows from our assumption that $D$ is the average of marginals of $D^{(m)}$. In a similar fashion, one can appropriately replace \eqref{eq:16}.

\subsection{Radamacher complexity.}

\yuval{Move the comments to the main body.}

Given a sample $S = (s_1, \dots, s_m) \in Z^m$, the 
\emph{$\rv{\tau}$-complexity} of $\cF$ with respect to the sample $S$ by:
\[
	\eRad_{S}^{\rv{\tau}}(\cF)
	= \EE_{\rv{\tau}} \left[ \sup_{f \in \cF}
	\sum_{i=1}^m \rv{\tau}_i f(s_i).
	\right],
\]

\emph{Radamacher complexity} of $\cF$ with respect to $S$ is defined as
\[
\eRad_{S}(\cF)
= \EE_{\rv{\sigma}} \left[ \sup_{f \in \cF}
\sum_{i=1}^m \rv{\sigma}_i f(s_i)
\right],
\]
where $\rv{\sigma} \in \{-1,1\}^m$ is a random vector of $m$ i.i.d unbiased coin flips. Note that in the usual definition, this term is  multiplied by $1/m$, which we avoid here for convenience. We generalize the notion of a Radamacher complexity, replacing the i.i.d signs with an arbitrary random variable $\rv{\tau} \in \mathbb{R}^m$. Define the \emph{$\rv{\tau}$-complexity} of $\cF$ with respect to the sample $S$ by:
\[
\eRad_{S}^{\rv{\tau}}(\cF)
= \EE_{\rv{\tau}} \left[ \sup_{f \in \cF}
\sum_{i=1}^m \rv{\tau}_i f(s_i).
\right],
\]
A particular case of interest is the \emph{Gaussian complexity}, denoted by $\eGC_{S}(\cF) := \eRad_{S}^{\rv{g}}(\cF)$, where $\rv{g}$ is a multivariate Gaussian $N(0, \Id_m)$. Both the Radamacher complexity and the Gaussian complexity were defined by \cite{bartlett2002rademacher}, and \citet{tomczak1989banach} proved the following:
\[
c\eRad_S(\cF) \le \eGC_S(\cF) \le C \ln m ~\eRad_S(\cF),
\]
for some universal constants $c, C > 0$. \citet{bednorz2014boundedness}, in a paper published in the Annuls of Mathematics, resolved a longstanding open problem characterizing 
Furthermore, the standard proofs for bounding the Radamacher complexity, which are based on bounding the deviation of sums of signed independent random variables, can be applied on the Gaussian complexity as well: the sum of independent normal variables have the same sub-Gaussian tail, hence the same bounds apply. This also applies to proofs using chaining and covering numbers.

The \emph{distributional Radamacher complexity} of $\cF$ with respect to a distribution $P^{(m)}$ over $Z^m$ is defined by
\[
\Rad_{P^{(m)}}(\cF) := \EE_{\rv{S} \sim P^{(m)}}\left[ \eRad_{\rv{S}}(\cF) \right],
\]
and similarly, the distributional $\rv{\sigma}$-complexity $\Rad_{P^{(m)}}^{\rv{\sigma}}(\cF)$ and Gaussian complexity $\GC_{P^{(m)}}(\cF)$ are defined. When the samples are drawn i.i.d, the right hand side of \eqref{eq:17} is bounded by $\frac{2}{m} \Rad_{D^{(m)}}(\cF)$. In the paper, We show that when the samples are non-i.i.d, the corresponding term can be bounded in terms of the Gaussian complexity.

One can define the Radamacher complexity directly on any pair of a hypothesis class $H$ and a loss function $\ell \colon Y^2 \to \mathbb{R}$. It is simply defined by $\eRad_S(H ; \ell) := \eRad_S(\mathcal{L}_H)$, where $\mathcal{L}_H := \{ \ell_h \colon h \in H\}$. The other complexities are similarly defined.

%In most common cases, the Gaussian Radamacher is roughly equivalent to the signed Radamacher complexity, and is going to be $\Theta(\sqrt{|S|})$. We define some notion of a worst-case Gaussian Radamacher complexity, where the worst case is taken over all datasets $S$ of all sizes.
%Formally, the \emph{Gaussian Radamacher constant} of $\cF$ is defined as
%\[
%\Rad^g(\cF) := \sup_{S} \eRad^g_{S}(\cF) / \sqrt{|S|}.
%\]

\subsection{Subgaussian distributions and stochastic processes}

A joint distribution $P^{(m)}$ over $\mathbb{R}^m$ is a $K^2$-subGaussian if has subgaussian tails in any direction:
\begin{definition}
	A zero-mean distribution $P^{(m)}$ over $\mathbb{R}^m$ is a $K^2$-subGaussian if for any $\theta \in \mathbb{R}^n$ and any $t > 0$,
	\[
	\Pr_{\rv{w} \sim P^{(m)}}\left[ \sum_{i=1}^m \theta_i \rv{w}_i > t \right]
	\le 2 \exp \left( \frac{-t^2}{2 K^2 \sum_{i=1}^m \theta_i^2}\right).
	\]
\end{definition}

A \emph{stochastic process} is a collection of joint random variables, $\{\rv{w}_i \}_{i \in I}$, taking values in $\mathbb{R}$, with some (possibly infinite) index-set $I$. A basic quantity of interest when talking about stochastic processes is the supremum, and in particular, the expected supremum, $\EE \sup_{i \in I} \rv{w}_i$. We will be focusing on \emph{zero-mean} processes, namely, those which satisfy $\EE \rv{w}_i = 0$ for all $i \in I$. We present two important types of stochastic processes: Gaussian and subGaussian processes. A \emph{Gaussian} process is a stochastic process where the variables are jointly Gaussian, namely, for any finite $U \subseteq I$, the collection $\{\rv{w}_i \}_{i \in U}$ is a multivariate Gaussian variable. A \emph{subGaussian process} is a stochastic process for which $w_i - w_j$ is subGaussian for all $i,j \in I$. The following statement by \citet{talagrand1996majorizing} upper bounds the expected maximum of a subGaussian process by that of a corresponding Gaussian process:

\begin{theorem} \label{thm:majorizing-measure}
	Fix $I$ to be some index set and let $\{\rv{w}_i\}_{i \in I}$ and $\{\rv{g}_i\}_{i \in I}$ be subGaussian and Gaussian zero-mean processes, respectively. For any $i,j \in I$, let $\sigma_{ij}^2$ denote the variance of $\rv{g}_i - \rv{g}_j$. Assume that for any $i,j \in I$, $\rv{w}_i - \rv{w}_j$ is a $\sigma_{ij}^2$-subGaussian random variable. Then,
	\[
	\EE\left[ \sup_{i \in I} \rv{w}_i \right]
	\le C \EE\left[ \sup_{i \in I} \rv{g}_i \right],
	\]
	for a universal constant $C>0$.
\end{theorem}

\subsection{Ising models}

For any $i \in \{1, \dots, m\}$, fix a function $\varphi_i \colon W \to \mathbb{R}$ and for any pair $i < j \in [m]$, fix a function, $\psi_{ij} \colon W^2 \to \mathbb{R}$. Each function $\varphi_i$ is called a \emph{node-wise} potential, and each $\psi_{ij}$ is called a \emph{pairwise potential}. A pairwise distribution is any distribution of the form
\[
\Pr[(w_1, \dots, w_m)] \propto \prod_{i=1}^m e^{\varphi_i(w_i)}
\prod_{1 \le i < j \le m} e^{\psi_{ij}(w_i w_j)},
\]
for arbitrarily chosen potential functions. 
Note that when the pairwise potentials equal zero, this defines a product distribution of i.i.d entries.
Although the pairwise potentials $\psi_{ij}$ were defined only for $i < j$, we may use $\psi_{ji}$ to denote the same potential.

Let $P^{(m)}$ be the corresponding distribution, and define for any $i \ne j \in [m]$ the \emph{influence factor} $\beta_{i,j}(P^{(m)}) = \sup_{w_i, w_j \in W} |\psi_{ij}(w_i w_j)|$. Define the \emph{inverse temperature} of the distribution as $\beta(P^{(m)}) := \max_{i \in [m]} \sum_{j \ne i} \beta_{ij}$. If the inverse temperature is less than $1$, then we have McDiarmid's inequality.

\yuval{prove that it satisfies Dobrushin's condition.}
\begin{theorem} \label{thm:ising-pairwise}
	Fix a distribution $P^{(m)}$ over $W^m$ with inverse temperature $\beta(P^{(m)}) < 1$. Fix some function $f \colon W^m \to \mathbb{R}$ and let $\lambda_1, \dots, \lambda_m \in \mathbb{R}$ be positive numbers which satisfy
	\[
	\forall w, w' \in W^m \colon \quad
	|f(w) - f(w')| \le \sum_{i=1}^m \mathbbm{1}_{w_i \ne w'_i} \lambda_i.
	\]
	Then, for all $t > 0$,
	\[
	\Pr_{(\rv{w}_1,\dots,\rv{w}_m) \sim P^{(m)}}\left[
	|f(\rv{w}) - \EE[f(\rv{w})]| > t
	\right]
	\le 2\exp\left( -\frac{t^2 (1 - \beta(P^{(m)}))}{C \sum_{i=1}^m \lambda_i^2} \right)
	\]
	where $C > 0$ is an absolute constant.
	In particular, if $P^{(m)}$ is a zero-mean distribution over $\{-1,1\}^m$, then it is a $C / (1 - \beta(P^{(m)}))$-subGaussian.
\end{theorem}
